# Supplementary material for: Prefer Nested Segmentation to Compound Segmentation
Source: arXiv:1705.01643 ancillary file (2017-05-03)
Supplement: Supplementary file 1 [file SupplementMain.pdf]

Supplementary material for article:

# Prefer Nested Segmentation to Compound Segmentation


Haley D. Clark[†,1,2], Stefan A. Reinsberg[1], Vitali Moiseenko[3], Jonn Wu[1,4], and Steven D. Thomas[2].

[1]Department of Physics and Astronomy, University of British Columbia, Vancouver, BC, Canada.

[2]Department of Medical Physics, British Columbia Cancer Agency, Vancouver, BC, Canada.

[3]Department of Radiation Medicine and Applied Sciences, University of California – San Diego, La Jolla, California, USA.

[4]Department of Medicine, University of British Columbia, Vancouver, BC, Canada.

† Corresponding author: H. D. Clark, via http://www.halclark.ca/Contact.html.


- Disclaimer: the views expressed in this manuscript are our own and are not the official position of our employers or funders.

May 3, 2017

## How oblique should oblique cleaving planes be?

Oblique cleaving planes help reduce the problem of grid-plane alignment where many voxels (i.e., whole rows, columns, slices) cross the boundary of a sub-segment when the cleaving plane is moved a small amount, as can happen if some contour edges are collinear with the voxel grid. There is an optimal cleave plane orientation that can be written when sub-segment extents are known exactly. This direction maximizes the minimum spacing between voxel-plane distance, ensuring small changes in the plane position results in the smallest possible number of voxels crossing the plane at one time (e.g., minimizing spatial resonances)[1]. For example, on a planar Cartesian grid considering the origin and nearest-neighbours only the min-max angle for a line[2] (within $[0, \frac{\pi}{4}]$, but seven more angles are identical due to symmetry) is 26.56505°. Including next-nearest neighbours yields 18.43495°. (Both are shown in figure 1.) The ultimate sub-segment dimensions are not known beforehand, so the angle must be estimated. Unfortunately, even estimation is difficult and costly [1,2]. Figure 2) depicts the objective function which must be maximized for square regions of limited extent. To simplify the use of oblique planes in this work, the requirement of optimality was relaxed and a cyclic rotation of 22.5° between cardinal axes was used throughout. Results indicate it was appropriate for our data set. It is worth noting that in many cases the problem can be avoided somewhat by irregular tessellation (e.g., [3–5]) and resampling of the dosimetric grid.

[1]Incidentally, this angle also appears to minimize the maximum spacing.
[2]This angle comes from the solution of $2 \sin x = \cos x$ within $[0° : 45°]$.

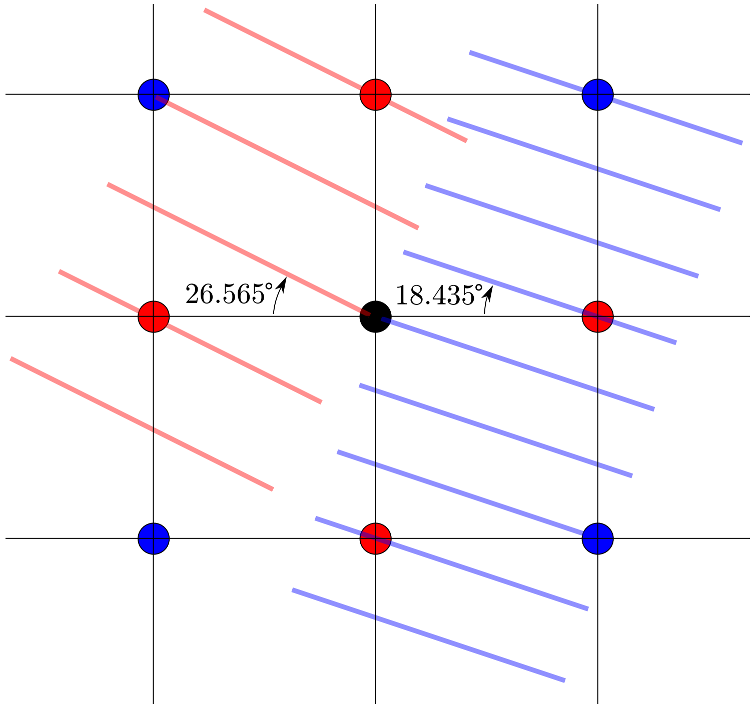


Figure 1: Depiction of voxel spacing at the min-max angle when nearest-neighbours (origin and red; red lines) and next-nearest-neighbours (origin, red, and blue; blue lines) are included. Figure 2 depicts how these angles are found.

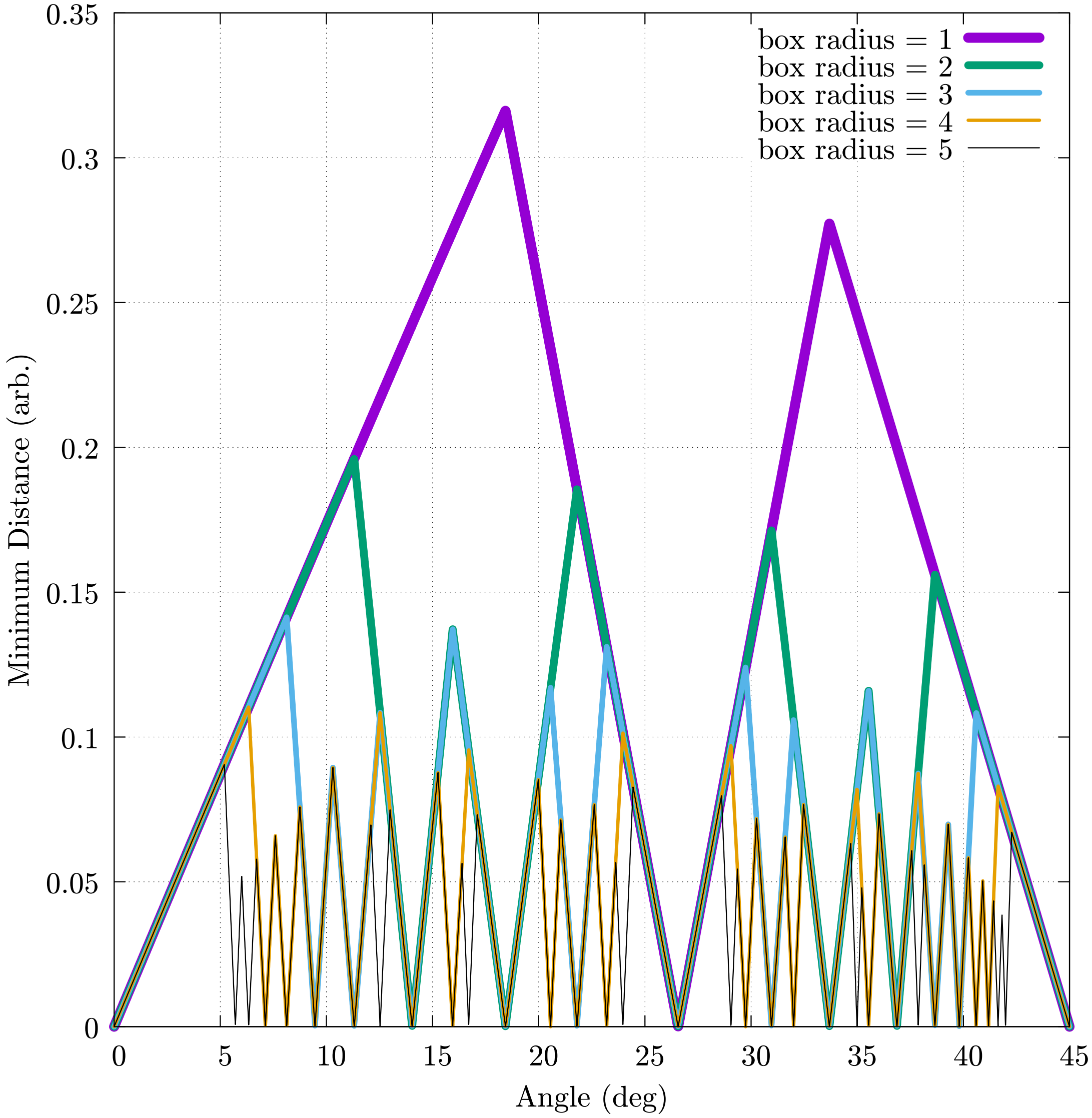


Figure 2: Minimum spacing between distances of voxel centres above line to line vs line angle for various box radii (i.e., a box of radius $n$ centred at the origin contains $(2n + 1)^2$ vertices). The next-nearest-neighbours example of fig. 1 corresponds to a box radius of 1. Grid spacing is $\Delta x = \Delta y = 1$ (arb. units). The min-max angle is the angle that maximizes this function. For square regions the left-most peak is maximal and shrinks as the box radius grows. For arbitrary geometry (e.g., ROIs) this is no longer generally true.

# References

[1] Fraser W. A Survey of Methods of Computing Minimax and Near-Minimax Polynomial Approximations for Functions of a Single Independent Variable. J ACM. 1965;12(3):295–314.

[2] Dem‘yanov VF, Malozemov VN. Introduction to minimax. Courier Corporation; 1974.

[3] Boots B, Okabe A, Sugihara K. Spatial tessellations. Geographical information systems. 1999;1:503–526.

[4] Tessellations UI. Hierarchical image analysis using irregular tessellations. IEEE transactions on pattern analysis and machine intelligence. 1991;13(4):307.

[5] Weatherill N. A method for generating irregular computational grids in multiply connected planar domains. International Journal for Numerical Methods in Fluids. 1988;8(2):181–197.
